# Supplementary material for: Estimating thresholds for asynchronous susceptible-infected-removed model on complex networks
Source: arXiv:2402.10863 source file (2024-02-16)
Supplement: Supplementary file 1 [file appendix1.tex]

\section{continuous approximation to transcendent equation } 
\label{appendix}

 Using continuous approximation to distribution probability \cite{alencar2023droplet}
 \begin{equation}
     P(k) = (\gamma-1)m^{\gamma-1}k^{-\gamma}/f(\gamma -1).
   \label{distrib-pln}
 \end{equation}

 Inserting \ref{distrib-pln} on \ref{transcendent} and integrating from $m$ to $k_{c}$ we obtain
 \begin{multline}
     \frac{ (\gamma-1)m^{\gamma-1}}{\langle k \rangle f(\gamma-1) } \lambda_{c}\left[\int_{m}^{\infty}\frac{k^{2-\gamma}}{k +\lambda_{c}}dk-\int_{k_{c}}^{\infty}\frac{k^{2-\gamma}}{k +\lambda_{c}}dk \right. \\
     -\left.\int_{m}^{\infty}\frac{k^{1-\gamma}}{k +\lambda_{c}}dk +\int_{k_{c}}^{\infty}\frac{k^{1-\gamma}}{k +\lambda_{c}}dk \right] = 1.
     \label{integral}
 \end{multline}

 Last expression is transformed to  Gauss hyper-geometric function $F(a,b,c;z)$\cite{gradshteyn2014table}
 \begin{multline}
     \frac{ (\gamma-1)m^{\gamma-1}}{\langle k \rangle f(\gamma-1)  } \lambda_{c}\left[\frac{\Gamma(\gamma-2) m^{2-\gamma}}{\Gamma(\gamma-1)} [F(1,\gamma-2,\gamma-1;-\lambda_{c}/m)\right.\\
     \left.-\left(\frac{k_{c}}{m}\right)^{2-\gamma}F(1,\gamma-2,\gamma-1;-\lambda_{c}/k_{c})]\right.\\
     -\left.\frac{\Gamma(\gamma-1) m^{1-\gamma}}{\Gamma(\gamma)}[F(1,\gamma-1,\gamma;-\lambda_{c}/m)\right. \\
     -\left.\left(\frac{k_{c}}{m}\right)^{1-\gamma}F(1,\gamma-1,\gamma;-\lambda_{c}/k_{c})]\right] = 1.
     \label{hypergeometric}
 \end{multline}
 
  Where $\Gamma(x)$ is the usual gamma function. Here, we can analyze the complete graph limit when $m\gg1$. Expansion to low orders in $z$ in last is made on power series \cite{gradshteyn2014table}
 \begin{equation}
     F(a,b,c;z) =1 + \frac{ab}{c}z + \frac{a(a+1)b(b+1)}{c(c+1)}z^{2} + \cdots .
     \label{hyper-expansion}
 \end{equation}

Applying eq. \ref{hyper-expansion} to \ref{hypergeometric} we have
\begin{multline}
     \frac{ (\gamma-1)m^{\gamma-1}}{\langle k \rangle f(\gamma-1)  } \lambda_{c}\left[\frac{\Gamma(\gamma-2) m^{2-\gamma}}{\Gamma(\gamma-1)}(f(\gamma-2)-\frac{(\gamma-2)}{\gamma-1}\frac{\lambda_{c}}{m}f(\gamma-1))\right.\\
     -\left.\frac{\Gamma(\gamma-1) m^{1-\gamma}}{\Gamma(\gamma)}(f(\gamma-1)-\frac{\gamma-1}{\gamma}\left(\frac{\lambda_{c}}{m}\right)f(\gamma)) + \mathcal{O(\lambda)}^{3}\right] = 1.
     \label{non-linear}
\end{multline}

Up to linear terms, we've, finally 
\begin{equation}
     \lambda_{c} \approx \frac{1}{1-\frac{(\gamma-2)f(\gamma-1)}{(\gamma-1)mf(\gamma-1)}} = \frac{\langle k \rangle}{\langle k \rangle-1}.
     \label{last}
\end{equation}
 And making the same approximation of eq. \ref{hpa} we obtain the same result on decay exponents $\epsilon_{1}$ and $\epsilon_{2}$ of eq. \ref{fitting-eq}. Thus, the HMF approximation is a partial term of the total solution, and heuristic approximation is interpreted as an effective solution for eq. \ref{non-linear}.%. Up to second order we've  from eq. \ref{non-linear}
 %\begin{equation}
     %\lambda^{2}_{c}\left[\frac{f -1}{\langle k %\rangle}\right] + \lambda_{c}/\lambda^{HMF}_{c} = 1,
 %\end{equation}
 %where $f= \langle 1/k \rangle$.
